# Supplementary material for: Single-collision statistics reveal a global mechanism driven by sample history for contact electrification in granular media
Source: arXiv:2211.02488 ancillary file (2023-03-20)
Supplement: Supplementary file 1 [file Suppl_info.pdf]

# Single-Collision Statistics Reveal a Global Mechanism Driven by Sample History for Contact Electrification in Granular Media: Supplemental Information

Galien Grosjean and Scott Waitukaitis  
*Institute of Science and Technology Austria (ISTA)*  
*Lab Building West*  
*Am Campus 1*  
*3400 Klosterneuburg AT*  
(Dated: January 26, 2023)

## EXPERIMENTAL SETUP

Levitation is achieved using acoustic forces, a technique which has the advantages of being manipulation-free and material-independent [38]. A Langevin ultrasonic transducer is fitted with a custom horn in which a spherical cap has been milled. It is held above a target substrate and powered by an amplifier using feedback circuitry to maintain the transducer in the desired current/phase regime, with a frequency  $f_T \approx 40$  kHz. When the distance between the horn and the substrate is a multiple of half the wavelength, a standing wave forms which can trap objects at the pressure node. The acoustic force on a small rigid sphere (radius  $R$ , density  $\rho$ , mass  $m$ ) in a plane standing wave of wavenumber  $k$  takes the form

$$F_A = -m \frac{5kp_0^2}{4\rho_0 c_0^2} \sin(2ky) = -ma \sin(2ky) \quad (\text{S1})$$

where  $\rho_0$  and  $p_0$  are the density and pressure of the air in the absence of the wave,  $c_0$  is the speed of sound, and  $a$  the acoustic amplitude [38]. Thanks to the curvature of the horn, the standing wave disappears progressively moving laterally outward, causing the sphere to be trapped horizontally as well. The left half of Fig. 1(a) of the main text shows a COMSOL simulation of the acoustic pressure amplitude inside the trapping volume.

To initiate a contact, we briefly interrupt the acoustic levitation, causing the sphere to fall on the substrate and bounce (Supplemental Video 1). Returning power to the transducer after the appropriate amount of time ( $\sim 25$  ms, at the apex of the bounce) allows us to catch the sphere again, which then oscillates around the equilibrium position at the resonant frequency of the trap  $f_{\text{trap}} \approx 50$  Hz [Fig. 1(b) of main text]. These oscillations dampen out over a timescale of seconds.

To measure charge, an electric field is applied accross the transducer gap so that the sphere experiences a Coulomb force (Supplemental Video 1). A copper electrode placed under the target substrate is connected to a high-voltage source, while the transducer horn is grounded. Using COMSOL, we plot the resulting electric field lines in Fig. 1(a) of the main text (right half), confirming they are close to what would be generated by a parallel-plate capacitor. As mentioned in the main text, we use the method proposed in [36] to measure charge. The key idea is to frequency sweep the electric field,  $E(t)$ , to pass through the natural frequency of the trap and record the resulting trajectory using a high-speed camera (Phantom VEO 640L). Newton's second law projected on the vertical direction can be written

$$\ddot{y} = -g + \frac{F_A}{m} + \frac{F_D}{m} + \frac{QE(t)}{m} = -g - a \sin 2ky - 2\beta_0 \dot{y} - 2\beta_1 |\dot{y}| \dot{y} + \frac{Q}{m} E_0 \sin \int_0^t \omega(t') dt' \quad (\text{S2})$$

where the unknowns are the acoustic amplitude,  $a$ , the linear and quadratic damping coefficients,  $\beta_0$  and  $\beta_1$ , and charge,  $Q$ . The electric field,  $E_0 \sin \int_0^t \omega(t') dt'$ , the acoustic wavenumber,  $k$ , and the sphere mass,  $m$ , are known, and the first and second derivatives  $\dot{y}$  can be calculated. A fifth fitting parameter,  $y_0$ , which corresponds to the sphere sagging due to gravity, is determined separately as in [36].

## ROTATION OF THE SPHERE

Due to their high sphericity and thorough cleaning, the rotation of our specimens can be hard to perceive as one must rely on the most minute defects and inhomogeneities. Supplemental Video 2 shows an instance where this is possible, due to a pair of barely visible specks of dust acquired after this sphere was left in the trap for 10+ days (an unusually long period). We use these specks to quantify rotation, as shown in Suppl. Fig. 1. First, we track the position of the sphere (orange cross) over time to remove extremely small ( $\sim 1 \mu\text{m}$ ) residual vibrations. We draw circles

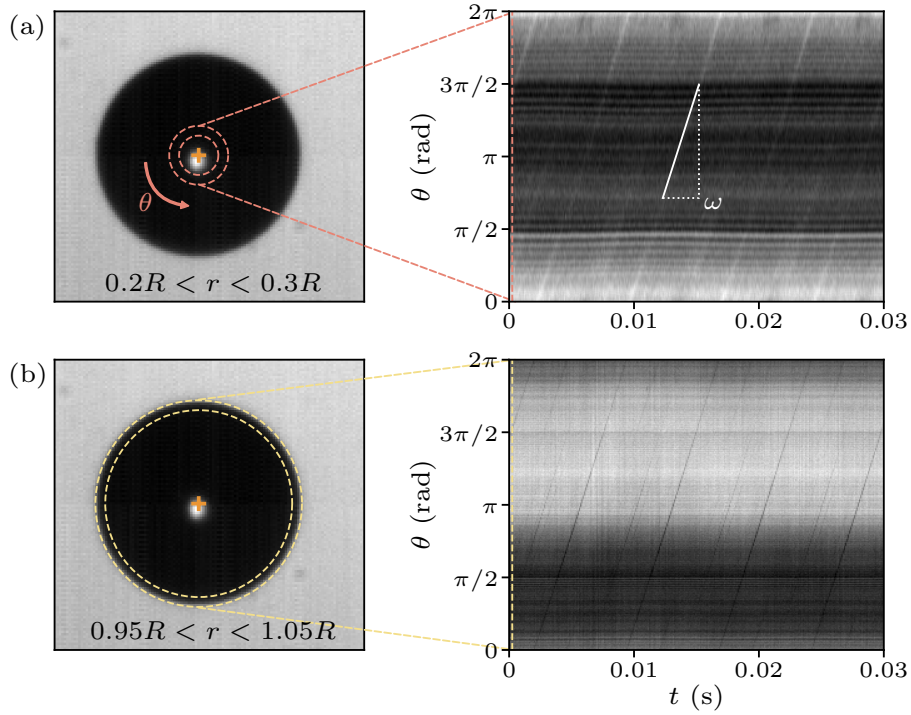

SUPPL. FIG. 1. Images (left) and rotation-time slices (right) showing the angular evolution over time of a levitating sphere. Two radial ranges are explored, (a) between 20 and 30 % of the total radius,  $R$ , and (b) between 95 and 105 % of  $R$ . Small inhomogeneities on the sphere rotate at a constant speed of around 900 rad/s, as evidenced by the diagonal lines in the rotation-time slices.

at constant radial distances from the sphere’s center, and then plot the temporal evolution of the image brightness as a function of the angle,  $\theta$ , between two such circles. Periodic features in this data are the signatures of angular motion.

The resulting rotation-time slices are shown for two radial ranges, in Suppl. Fig. 1(a) for  $0.2R < r < 0.3R$  and in Suppl. Fig. 1(b) for  $0.95R < r < 1.05R$ . Contrast has been increased to enhance features. Horizontal stripes on the slice are artifacts from the square pixel grid and imperfect lighting conditions. In both slices, however, we observe diagonal lines indicating that the sphere is rotating at an angular speed  $\omega \approx 900$  rad/s, or about 140 rotations per second. The rotation is approximately in the plane of the image in this case, though it need not be. Rotation speed and direction can vary substantially between spheres, and even over time for a given sphere. Given that the typical period of a rotation ( $2\pi/\omega \approx 1$  ms) is orders-of-magnitude smaller than the time between successive bounces ( $\approx 60$  s), we are ensured that the contact location on a sphere is randomly set for every collision.

## UNCERTAINTY IN CHARGE MEASUREMENTS

To characterize the experimental uncertainty in our charge measurements, we operate in ‘charge uncertainty mode,’ which consists of cycling over successive charge measurements at a particular  $Q$  without contacts or discharge (*ii*  $\rightarrow$  repeat). While levitating, charge decays over timescales of many days or even weeks [25, 39], hence the standard deviation of repeated charge measurements,  $\delta Q$ , taken over significantly shorter timescales (e.g. an hour) yields a robust estimate for the experimental uncertainty. Supplemental Figure 2(a) shows the relative uncertainty,  $\delta Q/Q$ , as a function of charge,  $Q$ . During our experiments, we modulate the electric field amplitude such that the maximum oscillation amplitude for any sweep remains approximately constant, regardless of the value of  $Q$ . For large values of  $Q$  ( $> 10^5$  elementary charges), this permits the relative uncertainty to be essentially constant, as the ratio of the oscillation amplitude to positional uncertainty can be maintained. For lower values of  $Q$ , we can no longer increase the amplitude of the electric field without reaching dielectric breakdown, thus resulting in smaller oscillation amplitudes with the same positional uncertainty, thus causing  $\delta Q/Q$  to increase. The relative uncertainty can be written as the

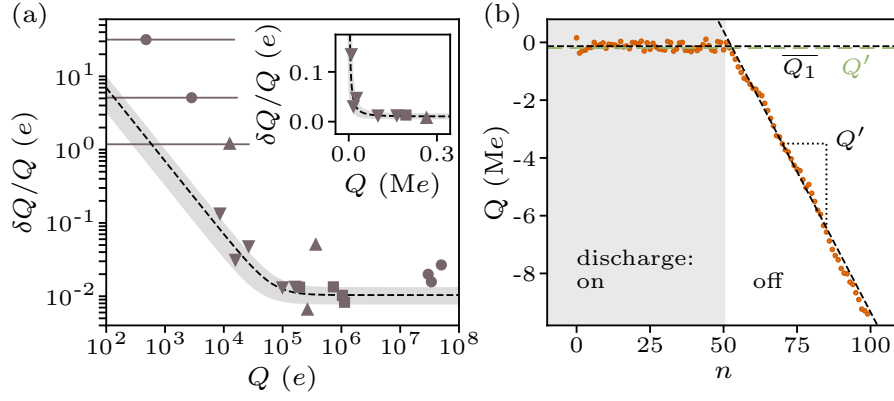

SUPPL. FIG. 2. (a) Relative uncertainty as a function of charge. Horizontal bars indicate one standard deviation. The inset shows some of the data on a linear scale. Different symbols correspond to different spheres. The fit is given by Suppl. Eq. (S3). (b) Sanity check between ‘charge distribution mode’ and ‘charge evolution mode.’ The former is employed for bounces 0-49, and the average,  $\overline{Q_1}$ , is indicated by the black dashed horizontal line. The latter is employed for bounces 50-100. The charging rate,  $Q'$  (green dashed horizontal line), lies essentially on top of  $\overline{Q_1}$ .

sum of a constant absolute value,  $\delta_c$ , and a constant relative value,  $\delta_r$ , so that

$$\delta Q = \sqrt{\delta_c^2 + \delta_r^2 Q^2}. \quad (\text{S3})$$

A fit on the data (dashed line) yields  $\delta_c \approx 700 e$  and  $\delta_r \approx 1\%$ . Considering that a typical amount of charge exchanged during a single contact is around  $10^5 e$ , individual contact events can therefore be resolved accurately, with an uncertainty of the order of  $\lesssim 10^3 e$ . Systematic biases also exist, which we estimate to be no more than  $\sim 3\%$  and come mainly from uncertainty on the sphere mass and electric field magnitude.

Related to the uncertainty issue, we sanity check in Suppl. Fig. 2(b) two experimental modes, namely ‘charge evolution mode’ and ‘charge distribution mode’. If the sphere is discharged before every contact using the photoionizer (first 50 contacts shown), the distribution of  $Q_1$  can be measured. On the other hand, when the discharging step is removed, the charge of the sphere is allowed to build up (contacts 50 to 100). The median value of the distribution  $\overline{Q_1}$  (black dashed horizontal line) is essentially the same as the rate  $Q'$  (green dashed horizontal line), indicating that the photoionizer has no effect on either measurement. However, discharging does provide the peace of mind that our distributions are produced from charging events that occur under the same conditions every measurement.

## DESCRIPTION OF SUPPLEMENTAL VIDEO 1

The three main tasks involved in our experimental modes are shown in succession in Supplemental Video 1, namely (i) contact, (ii) charge measurement and (iii) discharge. The contact is caused by a 26 ms interruption of the acoustic field. It was recorded originally at 25000 Hz and is shown here slowed down  $\times 50$ . For the charge measurement, an oscillating potential of 50 V was applied across the transducer gap, with the frequency increasing linearly from 10 to 100 Hz over 10 s. This video was recorded at 10000 Hz and is slowed down  $\times 2$ . During the discharge, a sinusoidal voltage of 60 V at 65 Hz was applied. The photoionizer is turned on after a few seconds, as indicated. The video was recorded at 500 Hz and is shown in real time.

## DESCRIPTION OF SUPPLEMENTAL VIDEO 2

Supplemental Video 2 shows the levitating sphere of Suppl. Fig. 1 over 1 s, slowed down  $\times 20$ . The original video was filmed at 10000 Hz. Some motion caused by vibrations can be seen, and one might also discern the rotation. This sphere had been levitating in the trap for more than 10 days when the video was taken, which explains why the two minuscule specks of dust that allows us to see the rotation are present. Naturally, we do not allow spheres to get this ‘dirty’ when we are taking charge measurements, which are done within a day or so of cleaning/baking.
